# Supplementary material for: Difference-in-Differences Estimators of Intertemporal Treatment Effects
Source: arXiv:2007.04267 source file (2026-05-12)
Supplement: Supplementary file 1 [file web_appendix2.pdf]

# Difference-in-Differences Estimators of Intertemporal Treatment Effects Web Appendix

Clément de Chaisemartin\*

Xavier D'Haultfoeuille†

## Abstract

In this web appendix, we consider several extensions to our theoretical results. In the first section, we propose parameters of interest and estimators for initially-treated groups. In the second section, we consider discrete treatments. In the third section, we consider continuous and staggered treatments. In the fourth section, we consider other extensions. Finally, the last section collects additional material on the application.

## 1 Initially-treated groups

In this section, we extend the analysis in Section 4 of the paper to groups that are treated at the first period. We thus consider designs where some initially-treated groups become untreated, at a date where some initially-treated groups have been treated all along, as stated below.

**Assumption 8** (*Non-pathological design for initially-treated groups*)  $\exists(g, g') \in \{1, \dots, G\}^2$  such that  $D_{g,1} = D_{g',1} = 1$  and  $F_g < F_{g'}$ .

### 1.1 Parameters of interest for initially-treated groups, and aggregated parameters

Let  $T_a = \max_{g: D_{g,1}=1} F_g - 1$  denote the last period where there is still a group that has been treated since period 1.  $T_a$  is the last period where initially-treated groups' treatment effects can be estimated under our assumptions. For any initially-treated group  $g$  such that  $F_g \leq T_a$ , and for any  $\ell \in \{0, \dots, T_a - F_g\}$ , let

$$\delta_{g,\ell} = E(Y_{g,F_g+\ell}(\mathbf{D}_g) - Y_{g,F_g+\ell}(\mathbf{1}) | \mathbf{D}) = E(Y_{g,F_g+\ell}(\mathbf{1}_{F_g-1}, 0, D_{g,F_g+1}, \dots, D_{g,F_g+\ell}) - Y_{g,F_g+\ell}(\mathbf{1}_{F_g+\ell}) | \mathbf{D}).$$

---

\*Economics Department, Sciences Po, clement.dechaisemartin@sciencespo.fr

†CREST-ENSAE, xavier.dhaultfoeuille@ensae.fr

$\delta_{g,\ell}$  is the expected difference between group  $g$ 's actual outcome at period  $F_g + \ell$ ,  $\ell$  periods after it got untreated for the first time, and the counterfactual "status quo" outcome it would have obtained at that period if it had remained treated from period one to  $F_g + \ell$ . For every  $g$ ,  $\delta_{g,\ell}$  is an effect of having received a weakly lower amount of treatment for  $\ell + 1$  periods. Depending on  $g$ 's treatments after period  $F_g$ ,  $\delta_{g,\ell}$  may correspond to the effect of having been untreated rather than treated from at least one to at most  $\ell + 1$  periods.

We can now define our main parameter of interest for initially-treated groups. In groups treated at period 1, the actual treatments are beneficial relative to the status quo, up to period  $T_a$ , if and only if

$$\sum_{g:D_{g,1}=1, F_g \leq T_a} \sum_{\ell=0}^{T_a-F_g} N_{g,F_g+\ell} \beta^{F_g+\ell} \delta_{g,\ell} - \sum_{g:D_{g,1}=1, F_g \leq T_a} \sum_{\ell=0}^{T_a-F_g} N_{g,F_g+\ell} \beta^{F_g+\ell} c_{g,\ell} (D_{g,F_g+\ell} - 1) > 0. \quad (36)$$

Let

$$c_- = \frac{\sum_{g:D_{g,1}=1, F_g \leq T_a} \sum_{\ell=0}^{T_a-F_g} N_{g,F_g+\ell} \beta^{F_g+\ell} c_{g,\ell} (1 - D_{g,F_g+\ell})}{\sum_{g:D_{g,1}=1, F_g \leq T_a} \sum_{\ell=0}^{T_a-F_g} N_{g,F_g+\ell} \beta^{F_g+\ell} (1 - D_{g,F_g+\ell})}$$

denote the average discounted cost of the treatment, across all the discounted treatments not received by groups initially treated. Assumption 8 ensures that  $c_-$ 's denominator is strictly positive. Dividing the left- and right-hand side of (36) by the negative of that denominator, we finally get that the actual treatments are beneficial up to period  $T_a$  if and only if

$$\delta_- := \frac{\sum_{g:D_{g,1}=1, F_g \leq T_a} \sum_{\ell=0}^{T_a-F_g} N_{g,F_g+\ell} \beta^{F_g+\ell} (-\delta_{g,\ell})}{\sum_{g:D_{g,1}=1, F_g \leq T_a} \sum_{\ell=0}^{T_a-F_g} N_{g,F_g+\ell} \beta^{F_g+\ell} (1 - D_{g,F_g+\ell})} < c_-. \quad (37)$$

Like  $\delta_+$ ,  $\delta_-$  can be written as an average total effect per unit of treatment. One may then average  $\delta_+$  and  $\delta_-$ , to form an average total effect per unit of treatment, across initially-untreated and initially-treated groups. Accordingly, let

$$\delta = w_+ \delta_+ + (1 - w_+) \delta_-,$$

where

$$w_+ = \frac{\sum_{g:D_{g,1}=0, F_g \leq T_u} \sum_{\ell=0}^{T_u-F_g} N_{g,F_g+\ell} \beta^{F_g+\ell} D_{g,F_g+\ell}}{\sum_{g:D_{g,1}=0, F_g \leq T_u} \sum_{\ell=0}^{T_u-F_g} N_{g,F_g+\ell} \beta^{F_g+\ell} D_{g,F_g+\ell} + \sum_{g:D_{g,1}=1, F_g \leq T_a} \sum_{\ell=0}^{T_a-F_g} N_{g,F_g+\ell} \beta^{F_g+\ell} (1 - D_{g,F_g+\ell})}.$$

The weight on  $\delta_+$  is proportional to the number of periods of exposure to treatment, among observations in initially-untreated groups. The weight on  $\delta_-$  is proportional to the number of periods of non-exposure to treatment, among observations in initially-treated groups.

Like  $\delta_+$ ,  $\delta_-$  is equal to a weighted average of event-study reduced-form effects, divided by a weighted average of event-study first-stage effects. Let  $L_a = T_a - \min_{g:D_{g,1}=1} F_g$  denote the difference between the last period at which a group has been treated all along and the earliest

period at which a group goes from treated to untreated. Under Assumption 8,  $L_a \geq 0$ . For every  $\ell \in \{0, \dots, L_a\}$ , let  $N_\ell^0 = \sum_{g: D_{g,1}=1, F_g \leq T_a - \ell} \beta^{F_g + \ell} N_{g, F_g + \ell} > 0$  be the discounted number of units in groups reaching  $\ell$  periods after their first untreated period at or before  $T_a$ . Let

$$\begin{aligned}\delta_{-, \ell} &= \sum_{g: D_{g,1}=1, F_g \leq T_a - \ell} \frac{\beta^{F_g + \ell} N_{g, F_g + \ell}}{N_\ell^0} (-\delta_{g, \ell}) \\ \delta_{-, \ell}^D &= \sum_{g: D_{g,1}=1, F_g \leq T_a - \ell} \frac{\beta^{F_g + \ell} N_{g, F_g + \ell}}{N_\ell^0} (1 - D_{g, F_g + \ell}).\end{aligned}\tag{38}$$

$\delta_{-, \ell}$  is the negative of the average effect of having switched treatment for the first time  $\ell$  periods ago, across all initially-treated groups that got untreated for the first time at least  $\ell$  periods before  $T_a$ .  $\delta_{-, \ell}$  is an effect of having experienced a weakly higher amount of treatment for  $\ell + 1$  periods.  $\delta_{-, \ell}^D$  is simply equal to one minus the average treatment of groups that got untreated for the first time  $\ell$  periods ago. Finally, let  $w_{-, \ell} = N_\ell^0 / \sum_{\ell'=0}^{L_a} N_{\ell'}^0$ . Following the same steps as those used to show Lemma 1, one can show that

$$\delta_- = \frac{\sum_{\ell=0}^{L_a} w_{-, \ell} \delta_{-, \ell}}{\sum_{\ell=0}^{L_a} w_{-, \ell} \delta_{-, \ell}^D}.\tag{39}$$

As  $\delta_{+, \ell}$  and  $\delta_{-, \ell}$  both measure the average effect of having been exposed to a weakly higher amount of treatment for  $\ell + 1$  periods, they may be aggregated. Let

$$\delta_\ell = \frac{N_\ell^1}{N_\ell^1 + N_\ell^0} \delta_{+, \ell} + \frac{N_\ell^0}{N_\ell^1 + N_\ell^0} \delta_{-, \ell}.$$

## 1.2 Identifying assumption and estimators for initially-treated groups

Let  $\mathbf{1}$  denote a  $1 \times T$  vector of ones. For initially-treated groups, our estimators rely on the following assumption on  $Y_{g,t}(\mathbf{1})$ , the always-treated potential outcome.

**Assumption 9** (*Independent groups, strong exogeneity, and parallel trends for always-treated outcome*)  $\forall t \geq 2$  and  $\forall g \in \{1, \dots, G\}$ ,  $E(Y_{g,t}(\mathbf{1}) - Y_{g,t-1}(\mathbf{1}) | \mathbf{D})$  does not vary across  $g$ .

Assumption 9 is the equivalent of Assumption 3, for the always-treated potential outcome. Together, Assumptions 3 and 9 imply that the effect of being always versus never treated follows the same evolution over time in every group:  $E(Y_{g,t}(\mathbf{1}) - Y_{g,t}(\mathbf{0}) | \mathbf{D}) - E(Y_{g,t-1}(\mathbf{1}) - Y_{g,t-1}(\mathbf{0}) | \mathbf{D})$  does not vary across  $g$ . Imposing jointly Assumptions 3 and 9 is necessary if one wants to estimate the treatment effects both for initially-treated and initially-untreated groups. If one only wants to estimate, say, the treatment effects for initially-untreated groups, imposing Assumption 3 is enough. Placebos similar to those defined in Section 4.3 of the paper could be proposed to test Assumption 9. They are omitted to preserve space.

We start by proposing conditionally unbiased estimators of the  $\delta_{g,\ell}$  parameters for initially-treated groups. Let  $N_t^a = \sum_{g:D_{g,1}=1, F_g > t} N_{g,t}$  denote the number of observations at period  $t$  in groups treated from period 1 to  $t$ . For every  $g$  such that  $D_{g,1} = 1$  and  $F_g \leq T_a$  and every  $\ell \in \{0, \dots, T_a - F_g\}$ , note that  $N_{F_g+\ell}^a > 0$ . Then, let

$$\text{DID}_{g,\ell} = Y_{g,F_g+\ell} - Y_{g,F_g-1} - \sum_{g':D_{g',1}=1, F_{g'} > F_g+\ell} \frac{N_{g',F_g+\ell}}{N_{F_g+\ell}^a} (Y_{g',F_g+\ell} - Y_{g',F_g-1}).$$

Following the same steps as those used to prove Lemma 2, one can show that if Assumptions 1-2 and 9 hold, then for every  $g$  such that  $D_{g,1} = 1$  and  $F_g \leq T_a$  and every  $\ell \in \{0, \dots, T_a - F_g\}$ , we have  $E[\text{DID}_{g,\ell} | \mathbf{D}] = \delta_{g,\ell}$ .

Then, we propose conditionally unbiased estimators of  $(\delta_{-, \ell})_{0 \leq \ell \leq L_a}$ , by replacing the  $\delta_{g,\ell}$  parameters by their estimators in Equation (38). Specifically, for every  $\ell \in \{0, \dots, L_a\}$ , let

$$\text{DID}_{-, \ell} = \sum_{g:D_{g,1}=1, F_g \leq T_a - \ell} \frac{\beta^{F_g+\ell} N_{g,F_g+\ell}}{N_\ell^0} (-\text{DID}_{g,\ell}). \quad (40)$$

We also propose a conditionally unbiased estimator of  $\delta_-$ , by replacing the  $\delta_{-, \ell}$  parameters by their estimators in Equation (39). Specifically, let

$$\hat{\delta}_- = \frac{\sum_{\ell=0}^{L_a} w_{-, \ell} \text{DID}_{-, \ell}}{\sum_{\ell=0}^{L_a} w_{-, \ell} \delta_{-, \ell}^D}.$$

Using similar arguments as those used to show Theorem 1 in the paper, one can show that the estimators  $(\text{DID}_{-, \ell})_{\ell \in \{0, \dots, L_a\}}$  and  $\hat{\delta}_-$  are conditionally unbiased under Assumptions 1-2 and 8-9

Turning to the parameters aggregating initially-untreated and initially-treated groups' effects, a conditionally unbiased estimator of  $\delta_\ell$  can be defined as

$$\text{DID}_\ell = \frac{N_\ell^1}{N_\ell^1 + N_\ell^0} \text{DID}_{+, \ell} + \frac{N_\ell^0}{N_\ell^1 + N_\ell^0} \text{DID}_{-, \ell}, \quad (41)$$

and a conditionally unbiased estimator of  $\delta$  can be defined as

$$\hat{\delta} = w_+ \hat{\delta}_+ + (1 - w_+) \hat{\delta}_-. \quad (42)$$

Our estimators for initially treated groups are computed by the `did_multiplegt` Stata package, when the `switchers(out)` option is specified. If the `switchers(in)` option is specified, estimators for initially untreated groups are computed. If no option is specified, aggregated estimators across initially treated and untreated groups are computed.

## 2 Discrete and potentially non-staggered treatments

### 2.1 Parameters of interest

In this section, we consider the case where the treatment is not binary, but ordered and discrete:  $\mathcal{D} = \{0, \dots, \bar{d}\}$  for  $\bar{d} \geq 1$ . For every  $g$ , let  $T_g = \max_{g': D_{g',1}=D_{g,1}} F_{g'} - 1$  denote the last period where there is still a group with the same treatment as  $g$ 's in period one and whose treatment has not changed since the start of the panel. For any  $g$  such that  $F_g \leq T_g$ , and for any  $\ell \in \{0, \dots, T_g - F_g\}$ , let  $\delta_{g,\ell} = E(Y_{g,F_g+\ell} - Y_{g,F_g+\ell}(D_{g,1}, \dots, D_{g,1}))$  be the expected difference between group  $g$ 's actual outcome at  $F_g + \ell$  and the counterfactual “status quo” outcome it would have obtained if its treatment had remained equal to its period-one value from period one to  $F_g + \ell$ .

We consider designs where Point 1 and either Point 2 or Point 3 (or both) in Assumption 10 below are met.

**Assumption 10** (*Non-pathological design for discrete treatments*)

1.  $\forall g \in \{1, \dots, G\}$ , either  $D_{g,t} \geq D_{g,1}$  for every  $t$ , or  $D_{g,t} \leq D_{g,1}$  for every  $t$ .
2.  $\exists (g, g') \in \{1, \dots, G\}^2$  such that  $D_{g,1} = D_{g',1}$ ,  $F_g < F_{g'}$ , and  $D_{g,F_g} > D_{g,1}$ .
3.  $\exists (g, g') \in \{1, \dots, G\}^2$  such that  $D_{g,1} = D_{g',1}$ ,  $F_g < F_{g'}$ , and  $D_{g,F_g} < D_{g,1}$ .

Point 1 requires that groups' treatments are either always weakly higher or always weakly lower than their period-one treatments. As discussed in the paper, for all  $(g, \ell)$  such that  $\ell$  periods after its first treatment change,  $g$  has experienced both a treatment strictly below and a treatment strictly above its period-one treatment,  $\delta_{g,\ell}$  can be written as a linear combination, with negative weights, of the effects of increasing the treatment at different periods. Accordingly,  $\delta_{g,\ell}$  could be negative even if increasing the treatment always increases the outcome. Under Point 1 of Assumption 10, such pairs  $(g, \ell)$  do not exist. If Point 1 fails, we recommend discarding such pairs  $(g, \ell)$ . This can be achieved easily, by discarding from the sample all cells  $(g, t)$  such that at  $t$ ,  $g$  has experienced both a treatment strictly below and a treatment strictly above its period-one treatment.

For all  $g$  such that  $F_g \leq T$ , let  $R_g = 1\{D_{g,F_g} > D_{g,1}\}$  be an indicator equal to 1 (resp. 0) for groups whose first treatment change is an increase (resp. a decrease). Under Point 1 of Assumption 10, groups with  $R_g = 1$  are such that  $D_{g,t} \geq D_{g,1}$  for all  $t$ , so  $\delta_{g,\ell}$  is an effect of having been exposed to a weakly higher amount of treatment for  $\ell + 1$  periods. Conversely, under Point 1, groups with  $R_g = 0$  are such that  $D_{g,t} \leq D_{g,1}$  for all  $t$ , so  $\delta_{g,\ell}$  is an effect of having been exposed to a weakly lower amount of treatment for  $\ell + 1$  periods.

Point 2 (resp. 3) of Assumption 10 requires that there is at least one group  $g$  experiencing a treatment increase (resp. decrease) at a time period where there is at least another group  $g'$  with

the same period-one treatment as  $g$  and whose treatment has not changed since the start of the panel. Point 2 (resp. Point 3) is sufficient to ensure that our parameters of interest for groups with  $R_g = 1$  (resp.  $R_g = 0$ ) are well-defined and can be unbiasedly estimated. Accordingly, Points 2 and 3 do not need to jointly hold to have that some of our estimators are applicable.

We now define our main parameter of interest, first for groups with  $R_g = 1$ . For several of the notation we introduce now, the quantity defined below coincides with a quantity already defined in the paper when the treatment is binary. In that case, we use the same notation here as in the paper. In groups with  $R_g = 1$ , the actual treatments are beneficial relative to the status quo, up to the last period where their treatment effects can be estimated, if and only if

$$\sum_{g: R_g=1, F_g \leq T_g} \sum_{\ell=0}^{T_g-F_g} N_{g, F_g+\ell} \beta^{F_g+\ell} \delta_{g,\ell} - \sum_{g: R_g=1, F_g \leq T_g} \sum_{\ell=0}^{T_g-F_g} N_{g, F_g+\ell} \beta^{F_g+\ell} c_{g,\ell} (D_{g, F_g+\ell} - D_{g,1}) > 0. \quad (43)$$

Let

$$c_+ = \frac{\sum_{g: R_g=1, F_g \leq T_g} \sum_{\ell=0}^{T_g-F_g} N_{g, F_g+\ell} \beta^{F_g+\ell} c_{g,\ell} (D_{g, F_g+\ell} - D_{g,1})}{\sum_{g: R_g=1, F_g \leq T_g} \sum_{\ell=0}^{T_g-F_g} N_{g, F_g+\ell} \beta^{F_g+\ell} (D_{g, F_g+\ell} - D_{g,1})}$$

denote the average discounted cost of the treatment, across all the incremental units of treatment received by groups with  $R_g = 1$  relative to their period-one treatment. Points 1 and 2 of Assumption 10 ensure that  $c_+$ 's denominator is strictly positive. Dividing the left- and right-hand side of (43) by that denominator, we finally get that the actual treatments are beneficial if and only if

$$\delta_+ := \frac{\sum_{g: R_g=1, F_g \leq T_g} \sum_{\ell=0}^{T_g-F_g} N_{g, F_g+\ell} \beta^{F_g+\ell} \delta_{g,\ell}}{\sum_{g: R_g=1, F_g \leq T_g} \sum_{\ell=0}^{T_g-F_g} N_{g, F_g+\ell} \beta^{F_g+\ell} (D_{g, F_g+\ell} - D_{g,1})} > c_+.$$

Here again,  $\delta_+$  can be written as an average total effect per unit of treatment.

Let  $L_u = \max_{g: R_g=1} (T_g - F_g)$  denote the largest  $\ell$  such that  $\delta_{g,\ell}$  can be estimated, for groups  $g$  such that  $R_g = 1$ . Under Point 2 of Assumption 10,  $L_u \geq 0$ . For every  $\ell \in \{0, \dots, L_u\}$ , let  $N_\ell^1 = \sum_{g: R_g=1, F_g \leq T_g - \ell} \beta^{F_g+\ell} N_{g, F_g+\ell} > 0$  be the discounted number of units in groups reaching  $\ell$  periods after their first treatment change at or before  $T_g$ . Let

$$\begin{aligned} \delta_{+, \ell} &= \sum_{g: R_g=1, F_g \leq T_g - \ell} \frac{\beta^{F_g+\ell} N_{g, F_g+\ell}}{N_\ell^1} \delta_{g,\ell}, \\ \delta_{+, \ell}^D &= \sum_{g: R_g=1, F_g \leq T_g - \ell} \frac{\beta^{F_g+\ell} N_{g, F_g+\ell}}{N_\ell^1} (D_{g, F_g+\ell} - D_{g,1}). \end{aligned} \quad (44)$$

Following the same steps as those used to show Lemma 1 in the paper, one can show that if Assumption 1 and Point 2 of Assumption 10 hold,

$$\delta_+ = \frac{\sum_{\ell=0}^{L_u} w_{+, \ell} \delta_{+, \ell}}{\sum_{\ell=0}^{L_u} w_{+, \ell} \delta_{+, \ell}^D}. \quad (45)$$

Parameters of interest can be defined symmetrically for groups with  $R_g = 0$ . Those definitions are omitted to preserve space.

## 2.2 Identifying assumption and estimators

For any  $d \in \mathcal{D}$ , let  $\mathbf{d}$  denote a  $1 \times T$  vector of  $ds$ . With a discrete treatment, our estimators rely on the following assumption on the potential outcomes  $Y_{g,t}(\mathbf{d})$ , that group  $g$  obtains at period  $t$  if its treatment is always equal to  $d$ .

**Assumption 11** (*Independent groups, strong exogeneity, and parallel trends for  $Y_{g,t}(\mathbf{d})$ -potential outcomes*)  $\forall d \in \mathcal{D}, \forall t \geq 2$ , and  $\forall g \in \{1, \dots, G\}$ ,  $E(Y_{g,t}(\mathbf{d}) - Y_{g,t-1}(\mathbf{d}) | \mathbf{D})$  does not vary across  $g$ .

Assumption 11 generalizes Assumption 3 to all the  $Y_{g,t}(\mathbf{d})$  potential outcomes. Placebos similar to those defined in Section 4.3 of the paper could be proposed to test Assumption 11. They are omitted to preserve space.

We start by proposing conditionally unbiased estimators of the  $\delta_{g,\ell}$  parameters. For all  $(g, t)$ , let  $N_t^g = \sum_{g': D_{g',1}=D_{g,1}, F_{g'} > t} N_{g',t}$  denote the number of observations at period  $t$  in groups  $g'$  with the same period-one treatment as  $g$ , and that kept the same treatment from period 1 to  $t$ . For every  $g$  such that  $R_g = 1$  and  $F_g \leq T_g$ , and every  $\ell \in \{0, \dots, T_g - F_g\}$ , we have  $N_{F_g+\ell}^g > 0$ . Then, let

$$\text{DID}_{g,\ell} = Y_{g,F_g+\ell} - Y_{g,F_g-1} - \sum_{g': D_{g',1}=D_{g,1}, F_{g'} > F_g+\ell} \frac{N_{g',F_g+\ell}}{N_{F_g+\ell}^g} (Y_{g',F_g+\ell} - Y_{g',F_g-1}).$$

$\text{DID}_{g,\ell}$  compares the  $F_g - 1$ -to- $F_g + \ell$  outcome evolution, in group  $g$  and in groups with  $g$ 's period-one treatment from period 1 to  $F_g + \ell$ . Using the same steps as those used to prove Lemma 2 in the paper, one can show that if Assumptions 1-2 and 11 hold, then for every  $g$  such that  $R_g = 1$  and  $F_g \leq T_g$  and every  $\ell \in \{0, \dots, T_g - F_g\}$ ,  $E[\text{DID}_{g,\ell} | \mathbf{D}] = \delta_{g,\ell}$ . Then, unbiased estimators of  $\delta_{+,\ell}$  can be formed by replacing  $\delta_{g,\ell}$  by  $\text{DID}_{g,\ell}$  in Equation (44). Similarly, an unbiased estimator of  $\delta_+$  can be formed by replacing the parameters  $\delta_{+,\ell}$  by their estimators in Equation (45).

## 3 Continuous and staggered treatments

Our approach can accommodate some continuous treatments. For instance, it is sometimes the case that  $D_{g,t} = I_g 1\{t \geq F_g\}$ , as in Proposition 3 in the paper: groups start getting treated at different dates, with potentially continuous group-specific intensities  $I_g$ , but once a group gets treated its treatment intensity never changes. The estimators we propose in Section 4 of the paper in the binary-treatment case for initially-untreated groups can still be readily used in that case. In this context, the parameter  $\delta_+$  is still a cost-benefit ratio comparing the actual and status-quo treatments of initially untreated groups. The interpretation of the parameters  $\delta_{+,\ell}$  slightly changes: those become average effects, across groups that become treated before period  $T_u - \ell$ , of having received  $I_g$  rather than 0 units of treatment for  $\ell + 1$  periods. By estimating

the first-stage effects  $\delta_{+,\ell}^D$ , one can assess the average value of  $I_g$  across those groups, which may help interpret the magnitude of  $\delta_{+,\ell}$ .

A frequent special case of staggered designs with a continuous treatment is when  $D_{g,t} = I_g 1\{t \geq F\}$ , as in Proposition 1 in the paper: there is no variation in treatment timing, only variation in treatment intensity. Again, the estimators we propose in Section 4 of the paper in the binary-treatment case for initially-untreated groups can still be readily used in that case, provided there are never-treated groups such that  $I_g = 0$ . Otherwise, there is no valid control group one may use to identify other groups' effects.

## 4 Other extensions

### 4.1 Controlling for covariates

Oftentimes, researchers want to control for a vector of covariates  $X_{g,t}$  in their estimation. In this section, we propose estimators controlling linearly for time-varying covariates. Another possibility would be to control for time-invariant covariates in a nonparametric way, following Callaway and Sant'Anna (2021). The two approaches rely on non-nested parallel trends assumptions and could in principle be combined. A practical advantage of the approach we propose is that it applies to the case where  $X_{g,t}$  is a vector of group-specific linear trends, a popular set of controls among applied researchers. The approach proposed in Callaway and Sant'Anna (2021) cannot accommodate group-specific linear trends.

We need to slightly modify our assumptions. Hereafter, we let  $\mathbf{X}_g = (X'_{g,1}, \dots, X'_{g,T})$  and  $\mathbf{X} = (\mathbf{X}_1, \dots, \mathbf{X}_G)$ .

**Assumption 12** (*Independence between groups, strong exogeneity and parallel trends with covariates for the never-treated outcome*) *There is a vector  $\theta_0$  of same dimension as  $X_{g,t}$  such that  $\forall(g, t), t \geq 2, E(Y_{g,t}(\mathbf{0}) - Y_{g,t-1}(\mathbf{0}) - (X_{g,t} - X_{g,t-1})'\theta_0 | \mathbf{D}, \mathbf{X})$  does not vary across  $g$ .*

Assumption 12 is similar to Assumption 3, except that it includes the covariates in the conditioning, and that the parallel trends assumption is on the “residualized” never-treated potential outcome  $Y_{g,t}(\mathbf{0}) - X'_{g,t}\theta_0$ . In de Chaisemartin and D'Haultfoeuille (2020), we showed that Assumption 12 underlies two-way fixed effects regressions with covariates. Assumption 12 requires that there exist  $\theta_0$  and  $\lambda_t$  such that

$$E(Y_{g,t}(\mathbf{0}) - Y_{g,t-1}(\mathbf{0}) | \mathbf{D}, \mathbf{X}) = (X_{g,t} - X_{g,t-1})'\theta_0 + \lambda_t.$$

Then, Assumption 12 allows for the possibility that groups experience different evolutions of their never-treated outcome over time, but it requires that those differential evolutions be accounted

for by a linear model in  $X_{g,t} - X_{g,t-1}$ , the change in a group's covariates. An interesting special case is when the control variables are group-specific linear trends. Then, Assumption 12 requires that

$$E(Y_{g,t}(\mathbf{0}) - Y_{g,t-1}(\mathbf{0})|\mathbf{D}) = \theta_{0g} + \lambda_t,$$

for some constants  $\theta_{0g}$  and  $\lambda_t$ . From  $t - 1$  to  $t$ , the evolution of the never-treated outcome in group  $g$  should deviate from its group-specific linear trend  $\theta_{0g}$  by an amount  $\lambda_t$  common to all groups. Then, Assumption 12 is a “common deviation from linear trends” assumption, which may be more plausible than the standard parallel trends assumption.

Let  $\hat{\theta}_0$  denote the coefficient of  $X_{g,t} - X_{g,t-1}$  in the OLS regression of  $Y_{g,t} - Y_{g,t-1}$  on  $X_{g,t} - X_{g,t-1}$  and time fixed effects, in the sample of all  $(g, t)$  such that  $F_{g,1} > t$ . For every  $g : D_{g,1} = 0, F_g \leq T_u$  and every  $\ell \in \{0, \dots, T_u - F_g\}$ , let

$$\begin{aligned} \text{DID}_{g,\ell}^X = & Y_{g,F_g+\ell} - Y_{g,F_g-1} - (X_{g,F_g+\ell} - X_{g,F_g-1})'\hat{\theta}_0 \\ & - \sum_{g': D_{g',1}=0, F_{g'} > F_g+\ell} \frac{N_{g',F_g+\ell}}{N_{F_g+\ell}^u} (Y_{g',F_g+\ell} - Y_{g',F_g-1} - (X_{g',F_g+\ell} - X_{g',F_g-1})'\hat{\theta}_0). \end{aligned}$$

$\text{DID}_{g,\ell}^X$  is similar to  $\text{DID}_{g,\ell}$ , except that instead of comparing groups' outcome evolution, it compares the part of that evolution that is not explained by a change in covariates.

Following the same steps as those used to prove Lemma 2, one can show that if Assumptions 1-2 and 12 hold, then for every  $g$  such that  $D_{g,1} = 1$  and  $F_g \leq T_u$ , and every  $\ell \in \{0, \dots, T_u - F_g\}$ , we have  $E[\text{DID}_{g,\ell}^X | \mathbf{D}, \mathbf{X}] = \delta_{g,\ell}$ . Then, conditionally unbiased estimators of  $(\delta_{+,\ell})_{0 \leq \ell \leq L_u}$  controlling for the covariates can be proposed, by replacing the  $\delta_{g,\ell}$  parameters by their estimators  $\text{DID}_{g,\ell}^X$  in Equation (8). Similarly, a conditionally unbiased estimator of  $\delta_+$  can be proposed, by replacing the  $\delta_{+,\ell}$  parameters by their estimators controlling for covariates in Equation (9). Using similar arguments as those used to show Theorem 1 in the paper, one can show that those estimators controlling for covariates are conditionally unbiased under Assumptions 1-2, 4, and 12. One can follow the exact same steps to propose placebo estimators to test Assumptions 2 and 12.

Our estimators controlling for covariates are computed by the `did_multiplegt` Stata package, when the `controls` option is specified. When the controls are group-specific linear trends, the `trends_lin` option needs to be specified.

## 4.2 Allowing for different trends across sets of groups

In some cases, controlling for covariates may be insufficient to account for differences in trends between groups. Then, a common remedy in static or dynamic two-way fixed effect regressions consists in including interactions between time FE and FE for sets of groups. For instance, if groups are US counties, one can allow for state-specific trends. A similar idea can be pursued

in our context. Let us index sets of groups by  $s \in \{1, \dots, S\}$ . In this set-up, we modify our assumptions as follows.

**Assumption 13** (*Parallel trends within sets of groups*) For all  $s \in \{1, \dots, S\}$ ,  $E(Y_{g,t}(\mathbf{0}) - Y_{g,t-1}(\mathbf{0}) | \mathbf{D})$  does not vary across  $g \in s$ .

Assumption 13 is a weakening of Assumption 3, as it only requires that the never-treated potential outcome of groups in the same set of groups follow the same evolution over time.

**Assumption 14** (*Non-pathological design, with parallel trends within sets of groups*)

1. There is at least one  $s \in \{1, \dots, S\}$  such that there exists  $(g, g') \in s^2$  such that  $D_{g,1} = D_{g',1} = 0$  and  $F_{g,1} < F_{g',1}$ .
2.  $T_u^s = \max_{g: D_{g,1}=0, g \in s} F_g - 1$  does not depend on  $s$ .

Point 1 of Assumption 14 requires that there is at least one set of groups within which an initially-untreated group gets treated for the first time at a date where another initially-untreated group is still untreated. Point 2 requires that the last period where at least one group has been untreated since the start of the panel be the same in every set of groups. This may hold when there are many never-treated groups, so that each set of groups may have at least one never-treated group. Outside of that case, this condition may be more restrictive. The only purpose of this condition is to ensure that under parallel trends within sets of groups, one can still unbiasedly estimate the parameters  $(\delta_{+, \ell})_{0 \leq \ell \leq L_u}$  and  $\delta_+$ , thus greatly alleviating the notational burden. If that condition fails, there are sets of groups for which  $\delta_{g, \ell}$  cannot be unbiasedly estimated for all  $\ell \in \{0, \dots, L_u\}$ , because  $T_u^s < T_u$ , so we would need to redefine the parameters  $(\delta_{+, \ell})_{0 \leq \ell \leq L_u}$  and  $\delta_+$ . This extension is conceptually straightforward but notationally burdensome. We omit it to preserve space.

For every  $s \in \{1, \dots, S\}$  and  $t \in \{1, \dots, T\}$ , let  $N_t^{u,s} = \sum_{g \in s: D_{g,1}=0, F_g > t} N_{g,t}$  denote the number of observations at period  $t$  in groups  $g \in s$  untreated from period 1 to  $t$ . For every  $s \in \{1, \dots, S\}$ , for every  $g \in s$  such that  $D_{g,1} = 0$  and  $F_g \leq T_u$ , and every  $\ell \in \{0, \dots, T_u - F_g\}$ , let

$$\text{DID}_{g,\ell}^s = Y_{g,F_g+\ell} - Y_{g,F_g-1} - \sum_{g' \in s: D_{g',1}=0, F_{g'} > F_g+\ell} \frac{N_{g',F_g+\ell}}{N_{F_g+\ell}^{u,s}} (Y_{g',F_g+\ell} - Y_{g',F_g-1}).$$

$\text{DID}_{g,\ell}^s$  is similar to  $\text{DID}_{g,\ell}$ , except that it only compares the outcome evolution of groups in the same set of groups  $s$ . For instance, if groups are US counties and sets of groups are US states,  $\text{DID}_{g,\ell}^s$  compares the outcome evolution of counties in the same state.

Following the same steps as those used to prove Lemma 2, one can show that if Assumptions 1-2 and 13-14 hold, then for every  $s \in \{1, \dots, S\}$ ,  $g \in s$  such that  $D_{g,1} = 0, F_g \leq T_u$  and  $\ell \in \{0, \dots, T_u - F_g\}$ , we have  $E[\text{DID}_{g,\ell}^s | \mathbf{D}] = \delta_{g,\ell}$ . Then, conditionally unbiased estimators of

$(\delta_{+, \ell})_{0 \leq \ell \leq L_u}$  relying only on parallel trends within sets of groups can be proposed, by replacing the  $\delta_{g, \ell}$  parameters by their estimators  $\text{DID}_{g, \ell}^s$  in Equation (8). Similarly, a conditionally unbiased estimator of  $\delta_+$  can be proposed, by replacing the  $\delta_{+, \ell}$  parameters by their estimators relying only on parallel trends within sets of groups in Equation (9). Using similar arguments as those used to show Theorem 1 in the paper, one can show that those estimators are conditionally unbiased under Assumptions 1-2 and 13-14. One can follow the exact same steps to propose placebo estimators to test Assumptions 2 and 13.

Our estimators relying on parallel trends within sets of groups are computed by the `did_multiplegt` Stata package, when the `trends_nonparam` option is specified.

### 4.3 Fuzzy designs

In this subsection, we briefly discuss fuzzy designs, where the treatment varies within  $(g, t)$  cells. The estimators we propose in this paper are readily applicable to groups that are fully untreated at period 1. Then, one just need to redefine the parameters  $(\delta_{+, \ell})_{0 \leq \ell \leq L_u}$  and  $\delta_+$ , replacing  $Y_{g, t}(\mathbf{D})$  by  $\frac{1}{N_{g, t}} \sum_{i=1}^{N_{g, t}} Y_{i, g, t}(\mathbf{D}_{i, g})$ , where  $\mathbf{D}_{i, g} = (D_{i, g, 1}, \dots, D_{i, g, T})$  is a vector stacking the treatments of observation  $i$  in group  $g$ . Then, one can show that under Assumptions 2-4,  $(\text{DID}_{+, \ell})_{0 \leq \ell \leq L_u}$  and  $\hat{\delta}_+$  are unconditionally unbiased for  $(\delta_{+, \ell})_{0 \leq \ell \leq L_u}$  and  $\delta_+$ .

In groups partly treated at period 1, the estimators proposed in this paper are not applicable. First, only groups where the proportion of treated units does not change over time can be used as controls, and such groups may not exist. When such groups exist, two estimation strategies, that differ from the ones considered in this paper, are available. First, one may separately estimate the outcome evolution of treated and untreated units in the control groups, and apply those counterfactual evolutions separately to treated and control units in groups whose proportion of treated units does change, and thus recover the counterfactual outcome those groups would have experienced if their proportion of treated units had not changed (see de Chaisemartin and D'Haultfœuille, 2018). Second, one may redefine the treatment as a continuous, group-level variable, and apply the estimators proposed by de Chaisemartin et al. (2022).

### 4.4 Ruling out lagged treatment effects

Up to now, we have made no restriction on the effects of past treatments. We now investigate the benefits of imposing such restrictions. Specifically, we consider the following assumption.

**Assumption 15-k** (*No effect of past treatments beyond  $k$  lags*)

For all  $(g, t)$ , all  $t$ , and all  $(d_1, \dots, d_t) \in \{0, 1\}^t$ ,  $Y_{g, t}((d_{t'})_{t' \leq t}) = Y_{g, t}(d_{t-k}, \dots, d_t)$ .

Assumption 15- $k$  is plausible when the treatment is unlikely to have very long-run effects. It is commonly made in event-study regressions and extensively discussed in Borusyak et al. (2021) and in Schmidheiny and Siegloch (2020) as a possible way to identify these regressions.

In our context, imposing Assumption 15 can provide a solution to the “initial conditions” problem. So far, we have assumed that the treatments prior to the start of the panel  $(D_{g,t})_{t \leq 0}$  do not affect potential outcomes. There are at least two situations where this assumption is innocuous. First, such treatments may not exist. Assume for instance that one seeks to estimate the effect of being unionized on earnings, using the NLSY panel. In this data set,  $t = 1$  corresponds to the first year on the labor market, so  $D_{g,t}$  is not defined for  $t \leq 0$ . Second, in staggered adoption designs, our main results still hold if potential outcomes depend on  $(D_{g,t})_{t \leq 0}$ . In groups  $g$  untreated at period 1,  $D_{g,t} = 0$  for all  $t \leq 0$ , so our results still hold. Outside of those designs, our results do not apply when potential outcomes depend on  $(D_{g,t})_{t \leq 0}$ . However, under Assumption 15- $k$ , our results apply to a restricted panel, including groups with a stable treatment from period 1 to  $k + 1$ , and starting at period  $k + 1$ . Note that a similar idea was already put forward by Schmidheiny and Siegloch (2020) in the context of event-study regressions, except that in the context of those regressions one only needs to drop the first  $k + 1$  periods of the panel, while we also need to drop groups whose treatment changes at some point between periods 1 and  $k + 1$ .

#### 4.5 First-difference placebo estimators

We now define the first-difference placebo estimators of Assumptions 2 and 3 discussed in Section 4.3 of the paper. First, for any  $g$  such that  $D_{g,1} = 0$  and  $3 \leq F_g \leq T_u$  and for any  $\ell \in \{0, \dots, F_g - 3\}$ , let

$$\text{DID}_{g,\ell}^{\text{fdp}} = Y_{g,F_g-1-\ell} - Y_{g,F_g-2-\ell} - \sum_{g': D_{g',1}=0, F_{g'} > F_g} \frac{N_{g',F_g}}{N_{F_g}^u} (Y_{g',F_g-1-\ell} - Y_{g',F_g-2-\ell}).$$

“fdp” stands for first-difference placebo.  $\text{DID}_{g,\ell}^{\text{fdp}}$  compares the outcome evolution of group  $g$  and of groups never treated from period 1 to  $F_g$ , between two consecutive periods,  $\ell + 1$  periods before  $g$  got treated. Let  $L_u^{\text{fdp}} = \max\{t \leq T_u : \exists g : F_g = t\} - 3$  denote the last time period at which a group switches from untreated to treated for the first time while there is still a group that has always been untreated, minus three. For every  $\ell \in \{0, \dots, L_u^{\text{fdp}}\}$ , let  $N_\ell^{1,\text{fdp}} = \sum_{g: F_g-3 \geq \ell} \beta^{F_g} N_{g,F_g} > 0$ , and let

$$\text{DID}_{+,\ell}^{\text{fdp}} = \sum_{g: F_g-3 \geq \ell} \frac{\beta^{F_g} N_{g,F_g}}{N_\ell^{1,\text{fdp}}} \text{DID}_{g,\ell}^{\text{fdp}}.$$

As with the long-difference placebos, one can show that if Assumptions 1-3 hold,

$$E \left[ \text{DID}_{+,\ell}^{\text{fdp}} \middle| \mathbf{D} \right] = 0 \quad \forall \ell \in \{0, \dots, L_u^{\text{fdp}}\}.$$

First-difference placebos are computed by the `did_multiplegt` Stata package, when the `placebo` option is specified. If the `longdiff_placebo` is also specified, the command instead computes the long-difference placebo estimators defined in Section 4.3 of the paper.

## 5 Supplementary results on the reanalysis of Favara and Imbs (2015)

This section collects supplementary results on our reanalysis of Favara and Imbs (2015).

First, Table 1 below shows the coefficients from a distributed-lag TWFE regression of the logarithm of loans volume on county and year fixed effects, the current treatment, and seven lags of the treatment, controlling for state-specific linear trends. All coefficients are small and statistically insignificant.

Table 1: Coefficients from distributed-lag TWFE regression of the logarithm of loans volume on banking deregulation

|                              |                     |
|------------------------------|---------------------|
| Period- $t$ deregulation     | -0.0443<br>(0.0504) |
| Period- $t - 1$ deregulation | -0.0177<br>(0.0578) |
| Period- $t - 2$ deregulation | -0.0280<br>(0.0498) |
| Period- $t - 3$ deregulation | -0.0106<br>(0.0391) |
| Period- $t - 4$ deregulation | 0.0118<br>(0.0219)  |
| Period- $t - 5$ deregulation | 0.0120<br>(0.0160)  |
| Period- $t - 6$ deregulation | 0.0040<br>(0.0127)  |
| Period- $t - 7$ deregulation | 0.0005<br>(0.0120)  |

Notes: The table shows the coefficients from a distributed-lag TWFE regression of the logarithm of loans volume on county and year fixed effects, the current treatment, and seven lags of the treatment, controlling for state-specific linear trends. The regression is estimated using the 1994-2005 county-level panel data set constructed by Favara and Imbs (2015). Standard errors are estimated using 100 bootstrap replications clustered at the state level. The regression is weighted by the inverse of the number of counties per state as in Favara and Imbs (2015).

Second, we study the effect of banking deregulations on houses prices. The blue line on Figure 1 shows our DID estimates of the effect of a first banking-deregulation on the logarithm of houses prices.  $\text{DID}_{+,0} = 0.004$  (s.e.=0.004): in the year of the first deregulation, house prices increase by 0.4% more in counties that deregulate than in counties that do not, an insignificant difference. This effect builds up over time, and becomes significant at the 10% level after 3 years ( $\text{DID}_{+,3} = 0.045$ , s.e.=0.024) and at the 5% level after 4 years ( $\text{DID}_{+,4} = 0.073$ , s.e.=0.031). To the left of zero, the placebo estimates are much smaller than the actual estimates (all are below 0.006 in absolute value) and insignificant: an F-test cannot reject the null that all placebos are insignificant (p-value=0.642). The green line on Figure 1 shows estimates of  $(\delta_{+,\ell})_{\ell \in \{0, \dots, 7\}}$  using a distributed-lag TWFE regression of the logarithm of houses prices on county and year fixed effects, the current treatment, and seven lags of the treatment, controlling for state-specific linear trends. The TWFE- and DID-based estimates are close, and insignificantly different. The standard errors of the TWFE-based estimates are much larger than those of the DID-based estimates, and all the TWFE-based estimates are insignificant.

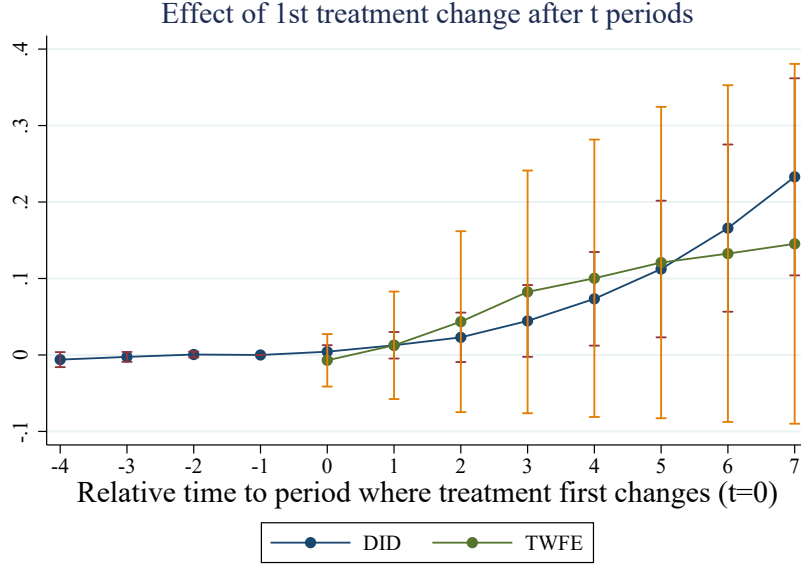

Figure 1: Effect of banking deregulations on housing prices.

Notes: To the right of zero, the blue line on the figure shows the  $DID_{+, \ell}$  estimates of the effect of a first banking-deregulation episode on the logarithm of house prices, the year of that first deregulation episode, and in later years. To the left of zero, the blue line shows the  $DID_{+, \ell}^{pl}$  placebo estimates. At  $x = -1$ , the placebo is normalized to 0.  $DID_{+, 0}^{pl}$  is shown at  $x = -2$ , etc. The estimates on the blue line are computed by the Stata `did_multipllegt` command, using the 1994-2005 county-level panel data set constructed by Favara and Imbs (2015). To the right of zero, the green line shows estimates of  $(\delta_{+, \ell})_{\ell \in \{0, \dots, 7\}}$  based on a distributed-lag TWFE regression of the logarithm of house prices on county and year fixed effects, the current treatment, and seven lags of the treatment. Standard errors are estimated using 100 bootstrap replications clustered at the state level. 95% confidence intervals relying on a normal approximation are shown in red for the  $DID_{+, \ell}$  and  $DID_{+, \ell}^{pl}$  estimates, and in orange for the TWFE estimates. Both sets of estimators have state-specific linear trends, and are weighted by the inverse of the number of counties per state as in Favara and Imbs (2015).

Combining the estimates shown on the blue line of Figure 1 to the first-stage estimated on Figure 2 in the paper leads to  $\hat{\delta}_{+, 0:7} = 0.037$  (s.e.=0.014). Across all deregulations, one deregulation increases house prices by 3.7% on average, when one sums the deregulation's instantaneous and dynamic effects. Even though this goes beyond the scope of this paper, one may tentatively divide the  $\hat{\delta}_{+, 0:7}$  estimator for housing prices by that for loan volume. Doing so, we obtain an elasticity of housing prices to loan volume of 0.137.

Third, we investigate whether differences between our specification and that in Favara and Imbs (2015) can explain why we reach such different conclusions. There are two differences between our specifications. First, their outcome variables are first-differences of the logarithm of loan volume and housing prices, while our outcome variables are in levels. Second, their treatment

variable is actually the lag of regulations in county  $g$ . We recompute our estimators mimicking their specification, and still find much larger long- than short-run effects. Figure 2 below shows the results for housing prices. Only six dynamic effects are shown, because the treatment is now lagged. Results are similar for loan volume.

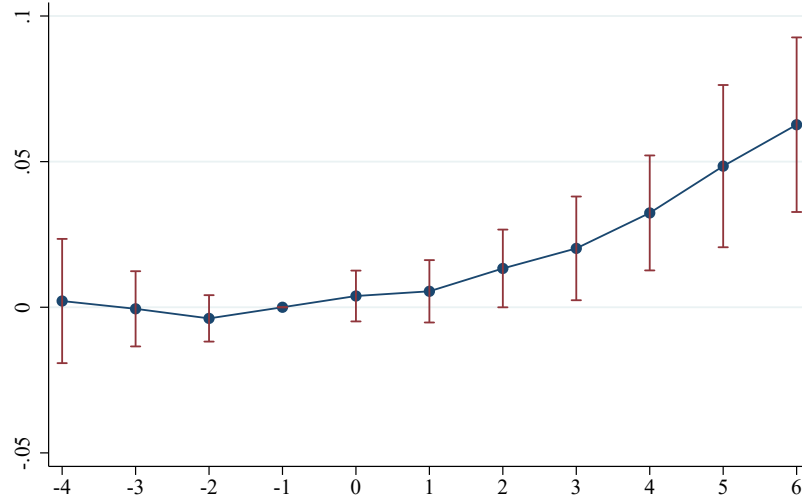

Figure 2: Effect of banking deregulations on housing prices, same specification as in Favara and Imbs (2015)

Notes: To the right of zero, the figure shows the  $DID_{+, \ell}$  estimates of the effect of the lag of a first banking-deregulation episode on the first difference of the logarithm of housing prices. To the left, the figure shows the  $DID_{+, \ell}^{pl}$  placebo estimates, that should not significantly differ from 0 if the parallel trends condition is satisfied. At  $x = -1$ , the placebo is normalized to 0.  $DID_{+, 0}^{pl}$  is shown at  $x = -2$ , etc. The estimates are computed by the Stata `did_multiplot` command, using the 1994-2005 county-level panel data set constructed by Favara and Imbs (2015). Standard errors are estimated using 100 bootstrap replications clustered at the state level. 95% confidence intervals relying on a normal approximation are shown in red. The estimation is weighted by the inverse of the number of counties per state as in Favara and Imbs (2015).

## 6 Details on the literature review

Table 2: List of highly-cited papers published by the AER from 2015 to 2019 using TWFE regressions

| Reference                       | Design                           | Estimate<br>dynamic effects? |
|---------------------------------|----------------------------------|------------------------------|
| Dell (2015)                     | Not binary and/or not staggered  | No                           |
| Burgess et al. (2015)           | Not binary and/or not staggered  | No                           |
| Favara and Imbs (2015)          | Not binary and/or not staggered  | Yes                          |
| Pierce and Schott (2016)        | Not binary and/or not staggered  | Yes                          |
| Hoynes et al. (2016)            | Binary, staggered                | Yes                          |
| Munshi and Rosenzweig (2016)    | Not binary and/or not staggered  | No                           |
| Atkin (2016)                    | Not binary and/or not staggered  | No                           |
| Allcott et al. (2016)           | Not binary and/or not staggered  | No                           |
| Suárez Serrato and Zidar (2016) | Not binary and/or not staggered  | Yes                          |
| Di Maggio et al. (2017)         | Binary, staggered                | Yes                          |
| Brandt et al. (2017)            | Not binary and/or not staggered  | No                           |
| Berman et al. (2017)            | Not binary and/or not staggered  | No                           |
| Handley and Limao (2017)        | Not binary and/or not staggered  | No                           |
| Dix-Carneiro and Kovak (2017)   | Not binary and/or not staggered  | Yes                          |
| Besley et al. (2017)            | Not binary and/or not staggered  | Yes                          |
| Donaldson (2018)                | Not binary and/or not staggered* | No                           |
| Fuest et al. (2018)             | Not binary and/or not staggered  | Yes                          |
| Hershbein and Kahn (2018)       | Not binary and/or not staggered  | Yes                          |
| Monte et al. (2018)             | Binary, staggered                | No                           |
| Huber (2018)                    | Not binary and/or not staggered  | No                           |
| Antecol et al. (2018)           | Binary, staggered                | Yes                          |
| Fetzer (2019)                   | Not binary and/or not staggered  | Yes                          |
| Kaur (2019)                     | Not binary and/or not staggered  | Yes                          |
| Naritomi (2019)                 | Binary, no variation in timing   | Yes                          |
| Bloom et al. (2019)             | Not binary and/or not staggered  | No                           |
| Diamond et al. (2019)           | Binary, no variation in timing   | No                           |

\*: Except in one table in the paper, where the treatment is binary and staggered.

## References

- Allcott, H., Collard-Wexler, A. and O’Connell, S. D. (2016), ‘How do electricity shortages affect industry? evidence from india’, *American Economic Review* **106**(3), 587–624.
- Antecol, H., Bedard, K. and Stearns, J. (2018), ‘Equal but inequitable: Who benefits from gender-neutral tenure clock stopping policies?’, *American Economic Review* **108**(9), 2420–41.
- Atkin, D. (2016), ‘Endogenous skill acquisition and export manufacturing in mexico’, *American Economic Review* **106**(8), 2046–85.
- Berman, N., Couttenier, M., Rohner, D. and Thoenig, M. (2017), ‘This mine is mine! how minerals fuel conflicts in africa’, *American Economic Review* **107**(6), 1564–1610.
- Besley, T., Folke, O., Persson, T. and Rickne, J. (2017), ‘Gender quotas and the crisis of the mediocre man: Theory and evidence from sweden’, *American economic review* **107**(8), 2204–42.
- Bloom, N., Brynjolfsson, E., Foster, L., Jarmin, R., Patnaik, M., Saporta-Eksten, I. and Van Reenen, J. (2019), ‘What drives differences in management practices?’, *American Economic Review* **109**(5), 1648–83.
- Borusyak, K., Jaravel, X. and Spiess, J. (2021), Revisiting event study designs: Robust and efficient estimation. arXiv preprint arXiv:2108.12419.
- Brandt, L., Van Biesebroeck, J., Wang, L. and Zhang, Y. (2017), ‘Wto accession and performance of chinese manufacturing firms’, *American Economic Review* **107**(9), 2784–2820.
- Burgess, R., Jedwab, R., Miguel, E., Morjaria, A. and Padró i Miquel, G. (2015), ‘The value of democracy: evidence from road building in kenya’, *American Economic Review* **105**(6), 1817–51.
- Callaway, B. and Sant’Anna, P. H. (2021), ‘Difference-in-differences with multiple time periods’, *Journal of Econometrics* **225**(2), 200–230.
- de Chaisemartin, C. and D’Haultfoeulle, X. (2018), ‘Fuzzy differences-in-differences’, *The Review of Economic Studies* **85**(2), 999–1028.
- de Chaisemartin, C. and D’Haultfoeulle, X. (2020), ‘Two-way fixed effects estimators with heterogeneous treatment effects’, *American Economic Review* **110**(9), 2964–2996.
- de Chaisemartin, C., D’Haultfoeulle, X., Pasquier, F. and Vazquez-Bare, G. (2022), Difference-in-differences estimators for treatments continuously distributed at every period. arXiv preprint arXiv:2201.06898.

- Dell, M. (2015), ‘Trafficking networks and the mexican drug war’, *American Economic Review* **105**(6), 1738–79.
- Di Maggio, M., Kermani, A., Keys, B. J., Piskorski, T., Ramcharan, R., Seru, A. and Yao, V. (2017), ‘Interest rate pass-through: Mortgage rates, household consumption, and voluntary deleveraging’, *American Economic Review* **107**(11), 3550–88.
- Diamond, R., McQuade, T. and Qian, F. (2019), ‘The effects of rent control expansion on tenants, landlords, and inequality: Evidence from san francisco’, *American Economic Review* **109**(9), 3365–94.
- Dix-Carneiro, R. and Kovak, B. K. (2017), ‘Trade liberalization and regional dynamics’, *American Economic Review* **107**(10), 2908–46.
- Donaldson, D. (2018), ‘Railroads of the raj: Estimating the impact of transportation infrastructure’, *American Economic Review* **108**(4-5), 899–934.
- Favara, G. and Imbs, J. (2015), ‘Credit supply and the price of housing’, *American Economic Review* **105**(3), 958–92.
- Fetzer, T. (2019), ‘Did austerity cause brexit?’, *American Economic Review* **109**(11), 3849–86.
- Fuest, C., Peichl, A. and Siegloch, S. (2018), ‘Do higher corporate taxes reduce wages? micro evidence from germany’, *American Economic Review* **108**(2), 393–418.
- Handley, K. and Limao, N. (2017), ‘Policy uncertainty, trade, and welfare: Theory and evidence for china and the united states’, *American Economic Review* **107**(9), 2731–83.
- Hershbein, B. and Kahn, L. B. (2018), ‘Do recessions accelerate routine-biased technological change? evidence from vacancy postings’, *American Economic Review* **108**(7), 1737–72.
- Hoynes, H., Schanzenbach, D. W. and Almond, D. (2016), ‘Long-run impacts of childhood access to the safety net’, *American Economic Review* **106**(4), 903–34.
- Huber, K. (2018), ‘Disentangling the effects of a banking crisis: Evidence from german firms and counties’, *American Economic Review* **108**(3), 868–98.
- Kaur, S. (2019), ‘Nominal wage rigidity in village labor markets’, *American Economic Review* **109**(10), 3585–3616.
- Monte, F., Redding, S. J. and Rossi-Hansberg, E. (2018), ‘Commuting, migration, and local employment elasticities’, *American Economic Review* **108**(12), 3855–90.

- Munshi, K. and Rosenzweig, M. (2016), ‘Networks and misallocation: Insurance, migration, and the rural-urban wage gap’, *American Economic Review* **106**(1), 46–98.
- Naritomi, J. (2019), ‘Consumers as tax auditors’, *American Economic Review* **109**(9), 3031–72.
- Pierce, J. R. and Schott, P. K. (2016), ‘The surprisingly swift decline of us manufacturing employment’, *American Economic Review* **106**(7), 1632–62.
- Schmidheiny, K. and Siegloch, S. (2020), On event studies and distributed-lags in two-way fixed effects models: Identification, equivalence, and generalization. ZEW Discussion Paper 20-01.
- Suárez Serrato, J. C. and Zidar, O. (2016), ‘Who benefits from state corporate tax cuts? a local labor markets approach with heterogeneous firms’, *American Economic Review* **106**(9), 2582–2624.
